# Supplementary material for: Laser-coolable polyatomic molecules with heavy nuclei
Source: arXiv:1610.08243 ancillary file (2017-06-22)
Supplement: Supplementary file 1 [file Supplementary-10i.pdf]

# Supplementary material to MS "Laser-coolable polyatomic molecules with heavy nuclei"

T.A. Isaev

*Petersburg Nuclear Physics Institute, Orlova Roscha. 1, 188300 Gatchina, Russia*

A.V. Zaitsevskii

*Petersburg Nuclear Physics Institute, Orlova Roscha. 1, 188300 Gatchina, Russia u*

*Chemistry Dept., M. Lomonosov Moscow State University, Moscow 119991, Russia*

E. Eliav

*School of Chemistry, Tel-Aviv University, 66978, Tel-Aviv, Israel*

## COMPUTATIONAL DETAILS OF EFFECTIVE CORE POTENTIAL, SPIN-FREE AND FULLY-RELATIVISTIC CALCULATIONS

*ARECP* Using the program package MOLPRO [1] Multiconfigurational Self-Consistent Field Hartree-Fock (MCSCF) calculations are performed for geometry optimization and normal mode analysis without symmetry restrictions for ground and first excited electronic states of RaOH. At first stage closed-shell Hartree-Fock calculations of the ground-state configuration of the singly charged molecular cation $RaOH^+$ are performed to obtain an initial guess for the molecular orbitals. For Ra energy-consistent Spin-Averaged Effective Core Potential (ARECP) with 78 electrons included in atomic core is used from MOLPRO ECP library [2]. Basis set supplied with ARECP is used for Ra atom [15s,14p,8d], while on O and H point-like nuclei the basis sets of AVTZ quality are used ([11s,6p,3d] on O and [6s,3p] on H). In the MCSCF calculations the electrons on first lowest molecular orbital (which is effectively 1s orbitral on O) were frozen, while 17 electrons were allowed to occupy any of the next 13 molecular orbitals. Orbitals 2−4 remained doubly occupied in all configurations. Thus in the MCSCF procedure 3920 determinants were forming 2352 Configuration State Functions (CSF's) to describe either ground or two excited near-degenerate electronic states. All three electronic states were optimized simultaneously with equal statistical weights. Subsequent computation of FC factors were performed with hotFCHT code [3–5] analogously to similar calculations in [6].

*SF/FS-RCCSD and DC/FS-RCCSD* In four-component calculations DIRAC program package is used [7] for the FS-RCCSD computations. The code is used both for calculations of the potential curves and TDMs in RaOH. Two basis sets on Ra were used in calculations of potential curves and TDM's (see Table I): 1) All-electron uncontracted Dyall's basis set of triple-zeta quality (v3z, [8]) [33s, 29p, 19d, 13f]. This basis set is spatially dense and allows best description of the ground electronic state. 2) Uncontracted ANO-RCC basis set of Roos et al [9] augmented with diffuse p- (exponent 0.002) and d- (exponent 0.010) functions, this basis size was [28s,26p,18d,12f]. This basis set is better suited for balanced calculations of both ground and excited electronic states and results with this basis set are provided in MS.

For light atoms basis sets of doule-zeta quality with polarization functions by Alrichs et al [10] are employed. The ground closed-shell state of $RaOH^+$ molecular cation has been chosen as the Fock-Space vacuum (sector (0,0)). Then additional electron was added to the six lowest-lying Kramers pairs, which form the active space in (0,1) sector of Fock space. Total active space includes the Kramers pairs of molecular orbitals with energy from -2.0 to 100 Hartree, thus 17 electrons are correlated in FS-RCCSD.

## COMPUTATIONAL DETAILS OF QUASI-RELATIVISTIC CALCULATIONS OF $\mathcal{P}$-ODD AND $\mathcal{P},\mathcal{T}$-ODD PARAMETERS

The computation scheme of $\mathcal{P}$-odd and $\mathcal{P},\mathcal{T}$-odd parameters is analogous to that used in [11, 12], so here we just outline the main stages of the computations. We used for Ra the same uncontracted Gaussian basis set with the exponent coefficients (EC) composed in the even-tempered manner as in [11]. For O and H basis sets of quadruple-zeta quality augmented with polarisation functions from TURBOMOLE basis set library(Turbomole-QZVPP) were used. The nuclear density was modelled by a spherical Gaussian distribution $\rho(R) = \rho_0 e^{-\frac{3}{2\xi}R^2}$, where $\xi$ is the mean root square radius of the corresponding nucleus computed according to the empirical formula $\xi = (0.836A^{1/3} + 0.57)$ fm $= (1.5798A^{1/3} + 1.077)\ 10^{-5}a_0$, where $A$ is taken equal 226 for Ra isotope. A modified version [11, 13–15] of the program package TURBOMOLE [16] was used for the complex generalised SCF (Hartree–Fock or Kohn–Sham) calculations. The value of $\mathcal{P}$-odd parameter $|W_\text{a}|$ was calculated according to the Eq. (3) from [11], and $\mathcal{P},\mathcal{T}$-

Таблица I: Basis sets of uncontracted Gaussians for SF/FS-RCCSD (Dyall's v3z) and DC/FS-RCCSD (augmented ANO- RCC) calculations .

| Dyall's v3z basis | | | | augmented ANO-RCC basis | | | |
|---|---|---|---|---|---|---|---|
| s | p | d | f | s | p | d | f |
| 5.80565570E+07 | 5.00564657E+07 | 5.73211611E+04 | 1.38629006E+03 | 54615913.6000000000 | 22902995.90000 | 12219.053000 | 787.39615700 |
| 1.54524704E+07 | 1.41078956E+07 | 1.37211900E+04 | 4.67836732E+02 | 13644310.6000000000 | 4560028.170000 | 5143.374790 | 365.04664600 |
| 5.28705247E+06 | 4.35017805E+06 | 4.54949200E+03 | 1.98496918E+02 | 4219580.9900000002 | 1106448.310000 | 2222.378040 | 175.49536000 |
| 2.01159919E+06 | 1.44751581E+06 | 1.80458301E+03 | 9.44903607E+01 | 1412175.8500000001 | 304836.7850000 | 988.070486 | 85.15822360 |
| 8.39348648E+05 | 5.11458884E+05 | 8.04257989E+02 | 4.76903467E+01 | 504524.4240000000 | 92710.0666000 | 449.738369 | 43.00080590 |
| 3.71281160E+05 | 1.90182872E+05 | 3.87334073E+02 | 2.49302970E+01 | 188914.8130000000 | 30701.9828000 | 212.704692 | 21.62348420 |
| 1.72944470E+05 | 7.40364943E+04 | 1.97153465E+02 | 1.30959204E+01 | 73701.6788000000 | 11019.2921000 | 103.893965 | 10.78370340 |
| 8.36497948E+04 | 3.01125681E+04 | 1.04071526E+02 | 6.79505201E+00 | 29665.5588000000 | 4275.1644700 | 52.165543 | 5.34211442 |
| 4.17673584E+04 | 1.28002327E+04 | 5.64127047E+01 | 3.35161155E+00 | 12219.0530000000 | 1780.8158300 | 26.452334 | 2.47131293 |
| 2.13502834E+04 | 5.69223184E+03 | 3.08907736E+01 | 1.38210100E+00 | 5143.3747900000 | 787.3961570 | 13.232805 | 0.98852517 |
| 1.11189842E+04 | 2.64671585E+03 | 1.67890972E+01 | 5.68426794E-01 | 2222.3780400000 | 365.0466460 | 6.604431 | 0.32139400 |
| 5.88090825E+03 | 1.28291666E+03 | 9.11756466E+00 | 2.12848990E-01 | 988.0704860000 | 175.4953600 | 3.098175 | 0.12855780 |
| 3.15917077E+03 | 6.44582958E+02 | 4.89199077E+00 | 9.75932963E-02 | 449.7383690000 | 85.1582236 | 1.430500 | |
| 1.72294310E+03 | 3.33762712E+02 | 2.55374053E+00 | | 212.7046920000 | 43.0008059 | 0.597098 | |
| 9.51443107E+02 | 1.76771530E+02 | 1.30158105E+00 | | 103.8939650000 | 21.6234842 | 0.241046 | |
| 5.29721346E+02 | 9.48098978E+01 | 6.38505218E-01 | | 52.1655431000 | 10.7837034 | 0.097309 | |
| 3.00187725E+02 | 5.19333028E+01 | 2.92330385E-01 | | 26.4523340000 | 5.3421144 | 0.039283 | |
| 1.72510500E+02 | 2.85329696E+01 | 1.09463920E-01 | | 13.2328053000 | 2.4713129 | 0.010000 | |
| 1.00277953E+02 | 1.53238118E+01 | 7.56605274E-02 | | 6.6044317000 | 1.1390980 | | |
| 5.86476426E+01 | 8.31968300E+00 | | | 3.0981751600 | 0.4183576 | | |
| 3.51299858E+01 | 4.38897906E+00 | | | 1.4305005600 | 0.1563284 | | |
| 2.09488964E+01 | 2.30318048E+00 | | | 0.5970985000 | 0.0625314 | | |
| 1.19638314E+01 | 1.17321581E+00 | | | 0.2539563900 | 0.0250125 | | |
| 7.11440168E+00 | 6.01525933E-01 | | | 0.1015825600 | 0.0100050 | | |
| 4.21057962E+00 | 2.97087111E-01 | | | 0.0406330200 | 0.0040020 | | |
| 2.34582823E+00 | 1.47749661E-01 | | | 0.0162532100 | 0.0020000 | | |
| 1.31510348E+00 | 6.00679983E-02 | | | 0.0065012800 | | | |
| 6.77422309E-01 | 2.77053641E-02 | | | 0.0026005100 | | | |
| 3.61549960E-01 | 1.24964369E-02 | | | | | | |
| 1.86223187E-01 | | | | | | | |
| 6.47483700E-02 | | | | | | | |
| 3.23951224E-02 | | | | | | | |
| 1.56556662E-02 | | | | | | | |

Таблица II: Calculated molecular parameters and FC factors for RaOH molecule. The results of DC/FS-RCCSD with Dyall's v3z and augmented RCC-ANO basis sets are provided. Also the results of FC factors calculations for RaX (X=OH) pseudomolecule are provided. Internuclear distances $R_i$ are given in Å and transition wavenumbers $T_e$ in inverse centimeters.

RaOH molecular parameters for DC/FS-RCCSD

| RCC-ANO basis | | | Dyall's basis | | |
|---|---|---|---|---|---|
| X ($^2\Sigma$) | $R_{(\text{Ra}-\text{X})}$ | 2.30 | A ($^2\Sigma_{1/2}$) | $R_{(\text{Ra}-\text{O})}$ | 2.40 |
| A ($^2\Pi$) | $R_{(\text{Ra}-\text{X})}$ | 2.29 | A ($^2\Pi_{1/2}$) | $R_{(\text{Ra}-\text{O})}$ | 2.38 |
| | $T_e$ | $12.6\times10^3$ | $T_e$ | | $12.2\times10^3$ |
| FC factors | 0.9470[a], 0.0519[b], 0.0011[c] | | FC factors | 0.9566[a], 0.04262[b] , 0.00078[c] | |
| $\sum$ | > 0.9999 | | $\sum$ | > 0.9999 | |

[a] $0_0^0$
[b] $1_1^0$ Ra–X stretching
[c] $1_2^0$ Ra–X stretching

odd parameter $W_s$ according to the Eqs. (2) – (4) from [17] (we note that due to typo the $\rho_A(\vec{r})$ member was omited in expression (2) in [17]). We have neglected the contributions from the light nuclei (O and H) to the considered molecular $\mathcal{P}$-odd and $\mathcal{P},\mathcal{T}$-odd properties, due to the strong dependence of these effects on the nuclear charge (see e.g. [11] and references therein). Though the expressions for $|W_a|$ and $W_s$ in [11] and [17] are derived for diatomic molecules, they are do applicable for any linear molecule too. We note that in the direct application of the present complex GHF/GKS approach only the absolute value of $W_a$ is immediately accessible, while for $W_s$ the sign is determined directly in the calculations.


[1] H.-J. Werner, P. J. Knowles, G. Knizia, F. R. Manby, and M. Schütz, WIREs Comput. Mol. Sci. **2**, 242 (2012).

[2] I. Lim, H. Stoll, and P. Schwerdtfeger, J. Chem. Phys. **124**, 034107 (2006).

[3] R. Berger and M. Klessinger, J. Comput. Chem. **18**, 1312 (1997).

[4] H.-C. Jankowiak, J. L. Stuber, and R. Berger, J. Chem. Phys. **127**, 234101 (2007).

[5] J. Huh and R. Berger, J. Phys. **380**, 012019 (2012).

[6] T. A. Isaev and R. Berger, http://arxiv.org/abs/1504.08326, Phys. Rev. Lett., 116, 063006 (2016).

[7] DIRAC, a relativistic ab initio electronic structure program, Release DIRAC15 (2015), written by R. Bast, T. Saue, L. Visscher, and H. J. Aa. Jensen, with contributions from V. Bakken, K. G. Dyall, S. Dubillard, U. Ekstroem, E. Eliav, T. Enevoldsen, E. Fasshauer, T. Fleig, O. Fossgaard, A. S. P. Gomes, T. Helgaker, J. Henriksson, M. Ilias, Ch. R. Jacob, S. Knecht, S. Komorovsky, O. Kullie, J. K. Laerdahl, C. V. Larsen, Y. S. Lee, H. S. Nataraj, M. K. Nayak, P. Norman, G. Olejniczak, J. Olsen, Y. C. Park, J. K. Pedersen, M. Pernpointner, R. Di Remigio, K. Ruud, P. Salek, B. Schimmelpfennig, J. Sikkema, A. J. Thorvaldsen, J. Thyssen, J. van Stralen, S. Villaume, O. Visser, T. Winther, and S. Yamamoto (see http://www.diracprogram.org).

[8] K. G. Dyall, J. Phys. Chem. A **113**, 12638 (2009).

[9] O. Roos, V. Veryazov, and P.-O. Widmark, Theor. Chem. Acc. **111**, 345 (2003).

[10] A. Schäfer, H. Horn, and R. Ahlrichs, J. Chem. Phys. **97**, 2571 (1992).

[11] T. A. Isaev and R. Berger, Phys. Rev. A **86**, 062515 (2012).

[12] T. Isaev and R. Berger, J. Molec. Spectrosc. **300**, 26 (2014), ISSN 0022-2852.

[13] R. Berger, N. Langermann, and C. van Wüllen, Phys. Rev. A **71**, 042105 (2005).

[14] R. Berger and C. van Wüllen, J. Chem. Phys. **122**, 134316 (2005).

[15] S. Nahrwold and R. Berger, J. Chem. Phys. **130**, 214101 (2009).

[16] R. Ahlrichs, M. Bär, M. Häser, H. Horn, and C. Kölmel, Chem. Phys. Lett. **162**, 165 (1989).

[17] T. A. Isaev and R. Berger, ArXiv e-prints (2013), 1302.5682.
